# Supplementary material for: Imperfect Is Perfect: Learned Column Prefilling for Branch-Price-and-Cut
Source: arXiv:2610.21001 source file (2026-10-14)
Supplement: Supplementary file 1 [file appendix.tex]

\clearpage
\makeatletter
\let\apx@orig@addcontentsline\addcontentsline
\def\addcontentsline#1#2#3{\def\apx@tempa{#1}\def\apx@tempb{toc}%
  \ifx\apx@tempa\apx@tempb\apx@orig@addcontentsline{apx}{#2}{#3}\else\apx@orig@addcontentsline{#1}{#2}{#3}\fi}
\section*{Contents of the appendix}
{\setcounter{tocdepth}{2}\@starttoc{apx}}
\makeatother
\numberwithin{equation}{section}
\makeatletter
\@ifundefined{proposition}{\newtheorem{proposition}{Proposition}[section]}{}
\@ifundefined{proof}{\newenvironment{proof}{\par\noindent\emph{Proof.}\ }{\hfill$\square$\par}}{}
\makeatother

\input{sections/app_bpc}
\input{sections/app_learning}
\input{sections/app_gpu}
\input{sections/app_results}
\input{sections/app_repro}
