# Supplementary material for: Imperfect Is Perfect: Learned Column Prefilling for Branch-Price-and-Cut
Source: arXiv:2610.21001 source file (2026-10-14)
Supplement: Supplementary file 2 [file appendixD_ablations.tex]

\input{sections/appD_tables}

Two ablations isolate the two learned components of Section~\ref{sec:method}: how the columns of a pool
should be supplied to column generation, and what the initial center of the smoothing rule should be.
Both use \appDOneInstN{} real instances of the main panel---X-set instances of the two deepest
route-size classes, long and very long. Every arm of an instance runs inside one job on one node,
bracketed by two vanilla solves; the vanilla column is the mean of the four vanilla solves of the two
brackets and is the denominator of every ratio in both tables; a run that times out, the limit being $1.5$ times the instance's first vanilla time plus $300$\,s, is reported as a lower bound ($\ge$); every completed arm reaches the same certified root bound as vanilla. Tables~\ref{tab:appD-pool}
and \ref{tab:appD-center} give the root times in seconds instance by instance, so that the reader sees
the raw measurements, and close with the instance-equal geometric mean of the ratio to vanilla; intervals are two-sided
$90$\,\% $t$ intervals on the log ratios.

\subsection{Supplying the columns: which pool, and how}
\label{app:results-pool}\label{app:pool}\label{sec:learn-pool}
\label{sec:exp-confirm}\label{app:confirm}\label{app:earlier}\label{app:results-earlier}\label{app:dose}\label{app:learnmore}

\paragraph{The folklore and its best evidence.}
Practitioners of column generation know the advice that pre-filling the master with heuristic columns
``does not help'': the LP starts wide, the first solve is slow, and the columns are thrown away again.
The two oracle arms of Table~\ref{tab:appD-pool} show where this experience comes from, and why it is only
half right. \textsc{Psupp} preloads exactly the support of the converged root LP---the routes with positive value in an optimal root solution, the best columns anyone could know in advance---and it is the worst arm of the
table: \appDOnePsuppCensoredN{} of the \appDOneInstN{} runs time out, and the five that finish are \appDOnePsuppGM$\times$ vanilla but still \appDOnePsuppOverPnGM$\times$ slower
than the deployed prefill on those instances (\textsc{Psupp}/\textsc{Pn}, \appDOnePsuppOverPnCI). A few perfect columns give the master a degenerate vertex to stand on and
nothing to move with. \textsc{Pconv}, which preloads the \emph{complete} column set of the converged
master, is the best arm at \appDOnePconvGM$\times$: what a pool has to
supply is not the optimum but a rich neighborhood of near-optimal routes. This is the sense in which
imperfect is perfect. Neither oracle is a method---both need a completed solve---but they mark two contrasting extremes of what a pool can supply, and on the deep XML instances of a preliminary experiment preloading a heuristic pool
(\initFullPoolGM$\times$, $n=\initFullPoolN$) or the converged basis (\initBasisGM$\times$) confirmed the
folklore rather than beating it (Section~\ref{sec:intro}).

\paragraph{Learning is necessary.}
\textsc{Pn} is the deployed prefill: the learned pool (Appendix~\ref{app:learning}) admitted lazily, the
mechanism of the next paragraph. \textsc{Ph} keeps that mechanism and replaces the learned pool by an
ordinary heuristic pool, one HGS run with one seed.

On the same instances and the same node the learned pool is \appDOnePhOverPnGM$\times$ faster
(\textsc{Ph}/\textsc{Pn}, 90\,\% interval \appDOnePhOverPnCI), and is the faster of the two on
\appDOnePnBeatsPhN{} of the \appDOnePhOverPnN{} instances.
The scorer lets the constructor propose an order of magnitude more feasible routes than one heuristic run
(\archivePnPoolRoutes{} against a few thousand on X-n1001-k43), and the archive is selective enough to
take only the ones that matter.

\paragraph{The steps we take are necessary.}
The deployed archive keeps the pool \emph{outside} the model: the master starts from the singleton initial
columns; after every LP re-solve the pool is priced under the current smoothed dual, the \archiveBatch{}
most negative routes are handed to the same admission check the pricers use, the labeling call of that iteration is skipped when at least one route is admitted, and the LP is re-optimized from the previous basis; a route is offered at most
once. One scan of the \archivePnPoolRoutes-route pool of X-n1001-k43 costs \archivePnScanMs{}\,ms; the
pool served the first \archivePnExclusiveIters{} iterations exclusively and \archivePnEverEnteredPct\% of
it ever entered the model. \textsc{Pdump} drops this discipline and places the whole learned pool in the initial master. On these instances no difference is detected between the lazy archive and the dump (\textsc{Pdump}/\textsc{Pn} \appDOnePdumpOverPnGM$\times$, interval \appDOnePdumpOverPnCI).
The gap is modest on these instances because the solver's column cleaner caps the live master at ten
thousand columns and repairs a wide start within a few iterations; it is the deep XML instances, where the
first barrier solve lands on a bad vertex, on which preloading costs \initFullPoolGM$\times$. The archive
costs nothing when preloading would have been harmless and saves the run when it would not, which is why
it is the deployed choice.

\begin{table}[h]
\centering\footnotesize\setlength{\tabcolsep}{2.5pt}
\caption{Supplying the columns: root time in seconds on the long and very-long X instances of the main panel, same job and node per row; $n$ customers, $K$ vehicles; \textsc{Pn} learned pool via the lazy archive (deployed), \textsc{Ph} HGS pool via the archive, \textsc{Pdump} the same learned pool preloaded, \textsc{Pconv}/\textsc{Psupp} oracles preloading the converged column set or its support; ``$\ge$'' marks a timed-out run.}
\label{tab:appD-pool}\label{tab:app-supply}
\begin{tabular}{lrrrrrrrr}
\toprule
instance & $n$ & $K$ & vanilla & \textsc{Pn} & \textsc{Ph} & \textsc{Pdump} & \textsc{Pconv} & \textsc{Psupp} \\
\midrule
\appDTabOneRowsNoPhdump
\midrule
\appDTabOneGMRowNoPhdump
\appDTabOneWinsRowNoPhdump
\bottomrule
\end{tabular}
\end{table}

\subsection{Choosing the center: the learned direction}
\label{app:results-center}\label{app:center}\label{sec:learn-center}
\label{app:results-centre}\label{sec:learn-centre-value}\label{sec:learn-direction}\label{sec:learn-model}\label{app:dircontrol}

The center model predicts the \emph{direction} of the converged root dual; the vector is then given a
magnitude and projected onto the structural box $\mathcal{B}=\{c:\ 0\le c_i\le\max(2d_{0i}-c_{\mathrm{veh}},0)\}$ of
\eqref{eq:install} (Appendix~\ref{app:learning}), and installed as the iteration-0 center of Wentges smoothing.
Table~\ref{tab:appD-center} tests this on the same instances with the center alone, no pool, as in the \emph{Center} column of Table~\ref{tab:ablation}.

\paragraph{Learning is necessary.}
\textsc{S} is the standard Wentges rule: no learned center, the solver seeds its own center at the end of
the first heuristic phase. The learned center \textsc{Cn}, the deployed model of Appendix~\ref{app:learn-centre-train}, is \appDTwoSOverCnGM$\times$ faster
(\textsc{S}/\textsc{Cn}, interval \appDTwoSOverCnCI), consistent with the panel-wide Center column of Table~\ref{tab:ablation}; standard smoothing alone recovers only \appDTwoSGM$\times$ of vanilla here.

\paragraph{The steps we take are necessary.}
\textsc{Crand} keeps the deployed magnitude, vehicle row and box projection but randomly permutes the
customer entries of the learned center---the direction is destroyed and nothing else. It costs
\appDTwoCrandOverCnGM$\times$ (\textsc{Crand}/\textsc{Cn}, \appDTwoCrandOverCnCI): the direction is what the smoothed pricing
queries inherit, and it is what the network learns. \textsc{Crand} still beats standard smoothing
(\appDTwoCrandGM$\times$ against \appDTwoSGM$\times$ of vanilla), so a calibrated center installed at
iteration $0$ is worth part of the gain by itself, and the learned direction adds the rest on top.

\begin{table}[h]
\centering\small\setlength{\tabcolsep}{5pt}
\caption{Choosing the center: root time in seconds on the instances and protocol of Table~\ref{tab:appD-pool}, center-only arms: \textsc{S} standard smoothing, \textsc{Crand} the learned center with its customer entries permuted, \textsc{Cn} the deployed center.}
\label{tab:appD-center}\label{tab:app-centres}
\begin{tabular}{lrrrrrr}
\toprule
instance & $n$ & $K$ & vanilla & \textsc{S} & \textsc{Crand} & \textsc{Cn} \\
\midrule
\appDTabTwoRows
\midrule
\appDTabTwoGMRow
\appDTabTwoWinsRow
\bottomrule
\end{tabular}
\end{table}

\subsection{Very short routes}
\label{app:results-veryshort}

\paragraph{Route-size classes.}
The XML generator \citep{queiroga2022xml} controls the average route size $r$, the expected number of
customers per route: $r$ is drawn uniformly from the range of the chosen class
(Table~\ref{tab:appD-routesize}), the demands $q_i$ from the chosen demand distribution, and the
capacity is set to $Q=\max\{\max_i q_i,\ \lceil r\sum_i q_i/n\rceil\}$ ($Q=\lfloor r\rfloor$ for
unitary demands), so that the minimum fleet $K_{\min}=\lceil\sum_i q_i/Q\rceil$ has about $n/r$
vehicles; the class is the fourth digit of the instance code. A Vrp-Set-X instance is assigned to the
class whose center, the mean of $n/K_{\min}$ over the XML300 and XML500 instances of that class, is
nearest to its own $n/K_{\min}$.

\begin{table}[h]
\centering\footnotesize\setlength{\tabcolsep}{6pt}
\caption{Route-size classes of the XML generator: the range of the average route size $r$ and the class name used in this paper.}
\label{tab:appD-routesize}
\begin{tabular}{lcccccc}
\toprule
class & 1 & 2 & 3 & 4 & 5 & 6 \\
\midrule
$r$ & $[3,5]$ & $[5,8]$ & $[8,12]$ & $[12,16]$ & $[16,25]$ & $[25,50]$ \\
name & very short & short & medium & long & very long & ultra long \\
\bottomrule
\end{tabular}
\end{table}

\paragraph{The very-short class.}
The main panel of Section~\ref{sec:experiments} starts at the short class. The very-short class was measured under the same protocol, five instances per set,
and Table~\ref{tab:appD-veryshort} reports it separately. Pricing is comparatively easy on these
instances: under the ng-route relaxation with memories of size $8$ (Appendix~\ref{app:bpc-cvrp}) the
pricer already returns many elementary routes, and since every prefilled column is an elementary
route, prefill has more to offer here than on the harder classes, bringing root pricing to
\ablVfourClassOnePnGM$\times$ vanilla on all \ablVfourClassOneInstN{} instances (best
\ablVfourClassOnePnBest$\times$). The dual direction the RMP produces is adequate on its own, so the
learned center adds no guidance and costs a little (Prefill+Center against Prefill
\ablVfourClassOneCentreOnPrefillGM$\times$, interval \ablVfourClassOneCentreOnPrefillCI), and exact
pricing is too small a share of the run for the GPU backend to matter (\ablVfourClassOneGGM$\times$).
Giving this class weight in the main panel would overstate the effect of prefill and hide the
bottleneck of the harder instances, which is why it is shown here as an outlier class rather than
pooled into Table~\ref{tab:ablation}.

\begin{table}[h]
\centering\footnotesize\setlength{\tabcolsep}{4pt}
\caption{Very short routes: geometric-mean root-time ratio to vanilla under the protocol of Table~\ref{tab:ablation}, with the number of instances faster than vanilla in parentheses.}
\label{tab:appD-veryshort}
\begin{tabular}{lrrrrr}
\toprule
Set & Inst. & Prefill & Center & GPU & Prefill+Center \\
\midrule
\ablTableVfourClassOneRowsWords
\midrule
\textbf{all} & \ablVfourClassOneInstN{} & \ablVfourClassOnePnGM{} (\ablVfourClassOnePnWins) & \ablVfourClassOneConlyGM{} (\ablVfourClassOneConlyWins) & \ablVfourClassOneGGM{} (\ablVfourClassOneGWins) & \ablVfourClassOneNcpuGM{} (\ablVfourClassOneNcpuWins) \\
\bottomrule
\end{tabular}
\end{table}
